# Supplementary material for: Effective permeability of an immiscible fluid in porous media determined from its geometric state
Source: arXiv:2208.08027 ancillary file (2023-06-22)
Supplement: Supplementary file 1 [file Supporting_Material.pdf]

# Effective permeability of an immiscible fluid in porous media determined from its geometric state

Fatimah Alzubaidi, Peyman Mostaghimi, Yufu Niu, and Ryan T. Armstrong\*

*School of Minerals and Energy Resources Engineering,  
University of New South Wales, Sydney, Australia*

Gelareh Mohammadi

*School of Computer Science and Engineering, University of New South Wales, Sydney, Australia*

James E. McClure

*National Security Institute, Virginia Tech, Blacksburg, VA, 24061, USA*

Steffen Berg

*Shell Global Solutions International B.V., Grasweg 31, 1031HW Amsterdam, The Netherlands*

(Dated: August 17, 2022)

Supporting materials include the following: (1) a derivation for the porous media friction factor and the corresponding effective permeability model, (2) details of the simulation cases conducted, (3) simulated geometric state data and corresponding effective permeabilities, and (4) artificial neural network training and optimisation.

## I. FRICTION FACTOR DERIVATION

The following is based on the works of Blake 1922 [1] and Kozeny 1927 [2] with further details provided by Bear 1988 [3] and Bird 2002 [4].

Consider a Newtonian fluid flowing through a porous domain. The domain has porosity,  $\phi$ , and pore volume,  $V_p$ . The fluid is incompressible,  $\nabla \cdot \mathbf{v} = 0$ . The flow is creeping at steady state conditions with no body force nor inertia, and thus the momentum balance reduces to  $\nabla \cdot \mathbf{\Pi} = \mathbf{0}$ , where  $\mathbf{\Pi}$  is the stress tensor.

The mechanical energy flux is  $\mathbf{v} \cdot \mathbf{\Pi}$ , whereby the divergence of the flux can be separated into three parts: (1) work done on a fluid element by changing its volume, (2) work done by mechanical dissipation, and (3) work done by motion of the element as a whole. Expressed as

$$\nabla \cdot (\mathbf{v} \cdot \mathbf{\Pi}) = -p\nabla \cdot \mathbf{v} + \Phi + \mathbf{v} \cdot (\nabla \cdot \mathbf{\Pi}). \quad (1)$$

Based on the constraints of an incompressible fluid and creeping flow, we have

$$\Phi = \nabla \cdot (\mathbf{v} \cdot \mathbf{\Pi}), \quad (2)$$

where  $\Phi$  is the rate of mechanical energy dissipation.

The total rate of mechanical energy dissipation per unit time within  $V_p$  is

$$E = \int_{V_p} \Phi dV, \quad (3)$$

where  $dV$  is a volume element of  $V_p$ .

From Equations 2 and 3 and applying the divergence theorem,

$$E = \int_S \mathbf{v} \cdot \mathbf{\Pi} \cdot d\mathbf{s}, \quad (4)$$

where  $S$  is the solid surface of an 'equivalent' domain and  $d\mathbf{s}$  is a directed element of surface area.

Given constant pressure,  $P$ , boundary conditions on the inlet and outlet face of the domain,

$$\Delta PA_c = \int_S \mathbf{v} \cdot \mathbf{\Pi} \cdot d\mathbf{s}, \quad (5)$$

where  $A_c$  is the cross-sectional area of the domain. Assuming that the domain is homogeneous along its length,

$$\Delta PA_c = \int_0^L \left[ \int_S \mathbf{v} \cdot \mathbf{\Pi} \cdot d\mathbf{s} \right] dz, \quad (6)$$

where the outer integral is simply  $L$ . The inner integral can be expressed as the total magnitude of the wall shear stress,  $\bar{\tau}S$ . Therefore,

$$\Delta PA_c = \bar{\tau}SL. \quad (7)$$

For a porous domain, hydraulic radius is commonly defined as the ratio of cross sectional area to the wetting perimeter,  $A_c/L$ . The standard definition of hydraulic radius ( $r_h$ ) for an 'equivalent' domain is

$$r_h = \frac{\phi D_p}{6(1 - \phi)}, \quad (8)$$

where  $D_p$  is particle (or grain) diameter and  $\phi$  is porosity.

The Fanning friction factor is defined as the ratio between the magnitude of the wall shear stress ( $\bar{\tau}$ ) and the kinetic energy.

$$f = \frac{\bar{\tau}}{(1/2)\rho U^2}, \quad (9)$$

---

\* Corresponding Author: ryan.armstrong@unsw.edu.au

where  $\rho$  is density and  $U$  is average velocity.

Based on Equations 7, 8, and 9, a porous media friction factor can be defined as

$$f_p = \frac{2r_h(\frac{\Delta P}{L})}{\rho U^2}. \quad (10)$$

However,  $U$  is written in terms of an average velocity, which is inconvenient for measuring flow through a porous domain. A volumetric flow rate ( $Q_i$ ) of phase  $i$  can be defined as

$$Q_i = U_i \phi A_c = U_{si} A_c, \quad (11)$$

where  $A_c$  is the cross-sectional area of the domain and  $U_{si}$  is the superficial velocity of phase  $i$ . Using  $U_{si}$ , we arrive at friction factor,  $f_p$ , as defined in Equation 1 of the manuscript.

To arrive at the linear relationship for the superficial phase velocity, i.e., Equation 3 in the manuscript. We postulate that the pressure drop-flow relationship for an 'equivalent' domain is similar to that for fully developed flow through a tube of arbitrary shape.

$$f = \frac{F(shapefactor)}{Re}, \quad (12)$$

where  $Re$  is Reynolds number and  $F(shapefactor)$  is a geometrical constant.

Reynolds number for porous media flow is commonly defined as

$$Re = \frac{U_{oi} D_p \rho}{\mu_i (1 - \phi)}, \quad (13)$$

where  $\mu_i$  is the viscosity of phase  $i$ .

Based on Equations ??, 12, and 13, we arrive at the linear relationship for the superficial phase velocity, i.e., Equation 3 in the manuscript.

## II. SIMULATION CASES AND IMAGE PROCESSING

In LBPM, the wetting of a surface to the two fluids present can be defined as a scalar affinity value ( $\phi$ ) ranging from -1 to +1. This is equivalent to treating the solid surface as an immobile phase with an affinity to the two fluids proportional to the distance of  $\phi$  to fluid -1 and fluid +1. For a flat surface of  $\phi$ , the static contact angle is

$$\cos(\theta) = \phi. \quad (14)$$

The model domain was generated using an X-ray microcomputed tomography (micro-CT) image of a North Sea sandstone. The image was collected at the Australian National University (ANU) and image processing was performed using the MANGO software developed at ANU [5, 6]. For mineral identification a thin

section of the rock was collected using scanning Electron Microscopy Energy Dispersive Spectroscopy (SEM-EDS) followed by Quantitative Evaluation of Materials by Scanning Electron Microscopy (QEMSCAN) software to determine the associated minerals [7].

A reservoir sandstone from the North Sea with porosity and permeability of 23% and 640 mD, respectively, was cored to 5 mm in diameter and 16 mm in length and solvent cleaned using toluene, methanol, and azeotropic chloroform/methanol, and then dried at 60°C [8, 9]. The rock was then imaged with micro-CT at a clean dry state at 2.3  $\mu$ m resolution with 100 kv X-ray energy over 22 hours. The rock was then cut perpendicular to its vertical length and prepared for 2D mineral mapping by resin impregnation followed by a series of polishing steps and lastly carbon coating [9]. An SEM-EDS instrument with QEMSCAN software was used for acquisition and mineral identification of the 2D thin section at 2.0  $\mu$ m resolution. The generated 2D mineral map was then registered to the 3D micro-CT tomogram [10]. 3D mineral segmentation of the micro-CT image was performed by distinguishing the X-ray intensity range of each mineral provided by registered 2D to 3D data sets. Minerals were segmented into seven groups: 1) Quartz and Na-plagioclase, 2) K-feldspar and Muscovite/Illite, 3) Kaolinite, 4) Siderite, 5) Mixed group, 6) Pyrite and 7) Zircon. The converging active contours algorithm which was used for segmentation mainly utilized the X-ray intensity of minerals and since Quartz and Na-plagioclase have similar X-ray attenuation, they cannot be discriminated. This is the same for the phase of K-feldspar and Muscovite. The mixed group was a mixture of Siderite, Apatite, Chlorite, Rutile and Ankerite.

TABLE I. Main minerals identified from QEMSCAN analysis. Volume fraction refers to the fraction of solid voxels that are a given mineral.

| Mineral                       | Volume Fraction |
|-------------------------------|-----------------|
| Kaolinite                     | 19%             |
| Quartz + Plagioclase (Silica) | 55%             |
| Feldspar+Illite/Muscovite     | 18%             |
| Ankerite, Chlorite and Rutile | 2.7%            |
| Siderite (carbonate)          | 3.6%            |
| Pyrite                        | < 1%            |
| Zircon                        | < 1%            |
| Unclassified                  | < 1%            |

The main minerals identified from QEMSCAN analysis are listed in Table I along with their corresponding volume fraction of solid grains. There are various papers in the literature that provide various contact angles for different minerals and fluid pairs. A brief summary of those that are relevant to this publication are provided in Table III. In particular, the contact angles for Quartz and Kaolinite appear to differ significantly depending on the specific fluids that the solid is in contact with. For simplification, we grouped the QEMSCAN minerals into three groups as explained in the main manuscript. These

groups were quartz, clay, and carbonate.

| Author | Mineral   | Fluids                    | $(\gamma_{ns} - \gamma_{ws})/\gamma_{wn}$ |
|--------|-----------|---------------------------|-------------------------------------------|
| [11]   | Quartz    | water-air                 | 4.1                                       |
|        | Quartz    | water/heptane             | 24.3                                      |
|        | Quartz    | water(PVP)/air            | 22.8                                      |
|        | Quartz    | water/heptane (quinoline) | 49.6                                      |
|        | Quartz    | water/heptane (CPC)       | 122.2                                     |
|        | Quartz    | CS <sub>2</sub> /water    | 172                                       |
| [12]   | Quartz    | water/air(n-propanol)     | 20                                        |
|        | Quartz    | water/air(methanol)       | 20                                        |
|        | Quartz    | water/air(cyclohexane)    | 19                                        |
|        | Quartz    | water/air(nitrobenzene)   | 30                                        |
|        | Quartz    | water/air                 | 17.4                                      |
| [? ]   | Kaolinite | water/hexane              | 53.3–116.0                                |
|        | Kaolinite | water/octane              | 56.9–120.5                                |
|        | Kaolinite | water/dodecane            | 61.4–123.5                                |
|        | Kaolinite | water/cis-decalin         | 68.3–128.1                                |
|        | Kaolinite | water/air                 | 17.4                                      |
| [13]   | Feldspar  | water/air                 | 13–23                                     |

To test a range of different wetting conditions, we assigned various affinity values to the different mineral groups. We tested various wetting conditions ranging from water-wet to various mixed-wet conditions as outlined in Table II. The wetting distribution was considered in three ways. (1) The mineral type is the only reason for the wetting affinity to vary. (2) Fluid history is the only reason for the wetting affinity based on an initial morphological drainage of the image to 20 percent saturation. (3) Wetting affinity varies based on both fluid history and mineral type.

TABLE II. Wetting conditions used for simulation.

| Wetting State       | Quartz | Clay | Carbonate |
|---------------------|--------|------|-----------|
| Water wet           | 0°     | 0°   | 0°        |
| Strong Intermediate | 30°    | 30°  | 30°       |
| Weak Intermediate   | 60°    | 60°  | 60°       |
| Quartz Wet          | 0.0°   | 120° | 120°      |
| Mixed Wet 1         | 20°    | 60°  | 60°       |
| Mixed Wet 2         | 20°    | 120° | 120°      |
| Mixed Wet 3         | 20°    | 120° | 60°       |
| Mixed Wet 4         | 60°    | 120° | 30°       |

The exact affinity values assigned to each simulation are provided in Table III.

### III. SIMULATED GEOMETRIC STATES

The simulations provided 25,906 unique morphological states, which are presented Fig. 1. The Euler characteristic trend for the (non-wetting phase) NWP followed the expected trend of increasing connectivity for more oil-wet conditions. The NWP stops percolating at high water saturation near Euler equal to one resulting in an effective permeability of zero at the corresponding saturation. The NWP surface area follows a linear trend with

TABLE III. Affinity values used for each simulation.

| Quartz (74%)<br>$(\gamma_{qn} - \gamma_{qw})/\gamma_{wn}$ | Kaolinite (19%)<br>$(\gamma_{kn} - \gamma_{kw})/\gamma_{wn}$ | Carbonate (6.3%)<br>$(\gamma_{cs} - \gamma_{cs})/\gamma_{wn}$ |
|-----------------------------------------------------------|--------------------------------------------------------------|---------------------------------------------------------------|
| -0.975995897315443                                        | -0.446778593584895                                           | -0.206236648838967                                            |
| -0.944009596016258                                        | -0.971016137860715                                           | -0.137439730577171                                            |
| -0.932781266514212                                        | 0.457413049880415                                            | 0.316811633761972                                             |
| -0.913537617307156                                        | 0.331226457376033                                            | -0.850183304864913                                            |
| -0.891287120059133                                        | -0.22355302516371                                            | 0.33666357723996                                              |
| -0.746523973532021                                        | -0.48465311806649                                            | 0.273710147477686                                             |
| -0.729964171536267                                        | -0.480893274769187                                           | -0.37726439954713                                             |
| -0.712016633246094                                        | 0.47594888182357                                             | -0.221909356769174                                            |
| -0.611155110411346                                        | -0.0149561855942011                                          | 0.209121339488775                                             |
| -0.607414650265127                                        | 0.827464802656323                                            | -0.0581634026020765                                           |
| -0.602254219353199                                        | -0.845936931204051                                           | 0.26621072134003                                              |
| -0.57490780390799                                         | 0.943483043462038                                            | -0.248990630265325                                            |
| -0.566431018058211                                        | 0.744531641248614                                            | -0.562139413319528                                            |
| -0.5120739354752                                          | 0.304665509611368                                            | -0.723551149014384                                            |
| -0.394090513233095                                        | 0.946559134870768                                            | 0.53245516307652                                              |
| -0.381530503276736                                        | 0.111255122348666                                            | 0.523976843804121                                             |
| -0.343924954067916                                        | 0.364346727728844                                            | 0.361812502611428                                             |
| -0.33389600738883                                         | -0.232813570648432                                           | 0.190617111045867                                             |
| -0.305555817205459                                        | 0.857006100937724                                            | 0.995698180049658                                             |
| -0.298090965952724                                        | 0.133286216296256                                            | 0.128129709511995                                             |
| -0.287126547191292                                        | -0.334490485489368                                           | -0.894931531045586                                            |
| -0.282209127210081                                        | -0.846874367445707                                           | 0.526142961811274                                             |
| -0.246982009615749                                        | 0.15594189427793                                             | 0.601268572732806                                             |
| -0.239406839944422                                        | 0.25852635409683                                             | -0.465798107907176                                            |
| -0.156780978664756                                        | 0.578306893352419                                            | 0.820544592104852                                             |
| 0.0352492337115109                                        | 0.736811962909997                                            | 0.9591508298181                                               |
| 0.0362598365172744                                        | -0.892407296225429                                           | 0.937855966854841                                             |
| 0.105785397347063                                         | -0.314748682547361                                           | -0.393419045954943                                            |
| 0.144622361287475                                         | -0.421423598192632                                           | -0.296301209367812                                            |
| 0.37360928254202                                          | 0.277930609416217                                            | -0.0302097788080573                                           |
| 0.492302694357932                                         | 0.678233273327351                                            | -0.984669730998576                                            |
| 0.515742613468319                                         | 0.838482574559748                                            | -0.667262552771717                                            |
| 0.586434461176395                                         | -0.222873904742301                                           | -0.232088832650334                                            |
| 0.830802406650037                                         | 0.778277463279665                                            | -0.25978610990569                                             |
| 0.879116127733141                                         | -0.483778777997941                                           | -0.778400439303368                                            |
| 0.912559895776212                                         | -0.713239821605384                                           | 0.847819402813911                                             |

saturation as observed by others for water-wet conditions and increasing non-linearity with oil-wet conditions. The constitutive relationships for capillary pressure and relative permeability were also well aligned with expected behaviours. Capillary pressure was positive for water-wet conditions and negative for more oil-wet conditions. The oil phase effective permeability increased for more water-wet conditions while the water phase relative permeability decreased resulting in a net effect of shifting the crossing point of the two curves to the right.

### IV. NETWORK TRAINING AND OPTIMISATION

We used an ANN to predict the effective permeability of the connected oil phase using the Minkowski functionals, as described in Equation 8 of the manuscript. The

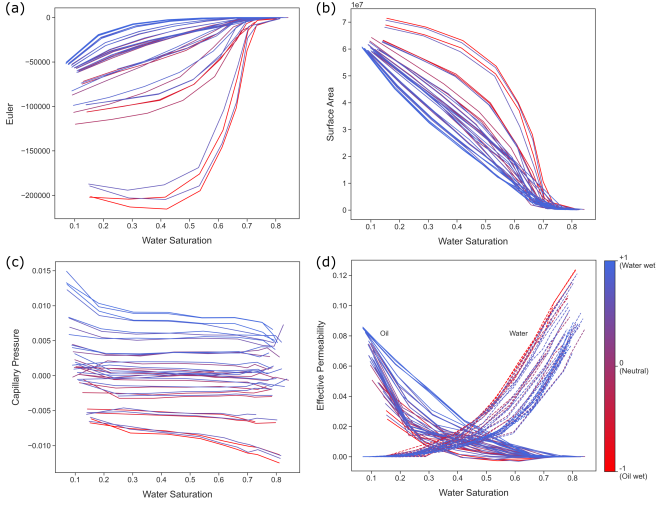

FIG. 1. Simulations provided 25,906 unique geometrical states (a,b) and corresponding capillary pressure (c) and relative permeability (d).

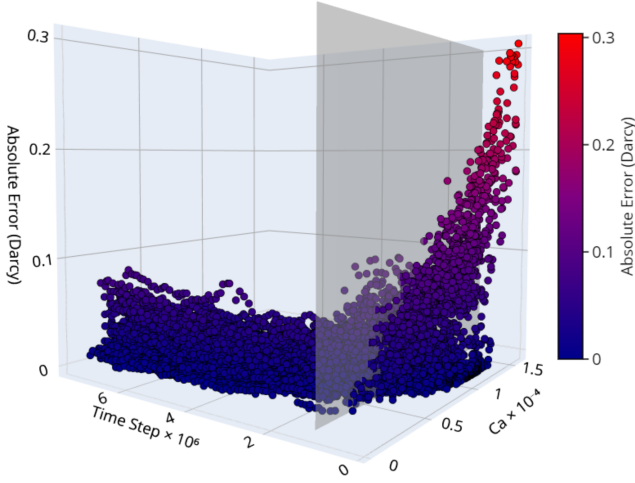

FIG. 2. Representative points from the simulation obtained after  $1 \times 10^6$  time steps (the grey plane). Data after this time step was used to build the ANN model presented in the main paper.

ANN model was optimized in terms of the input data and the network architecture and learning hyperparameters. The simulation provided a total of 25,906 data points. We found that representative points were obtained after the simulation convergence, which can be indicated by a convergence of Capillary number,  $Ca$ . Therefore, by visualizing  $Ca$  over simulation time in addition to the associated error for each point (see Figure 2), we have included points after  $1 \times 10^6$  time steps. The excluded points represent the earliest set recorded during the simulation as data was recorded every  $1 \times 10^6$  steps to up to  $78 \times 10^5$ . The remaining data, which include 22,556 points, was used to develop and evaluate the ANN. The data was divided randomly into train, validation, and

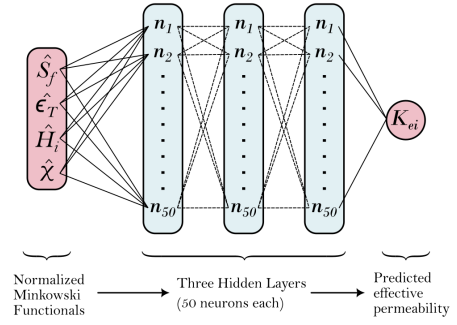

FIG. 3. An Artificial Neural Network of fully-connected layers for predicting effective permeability.

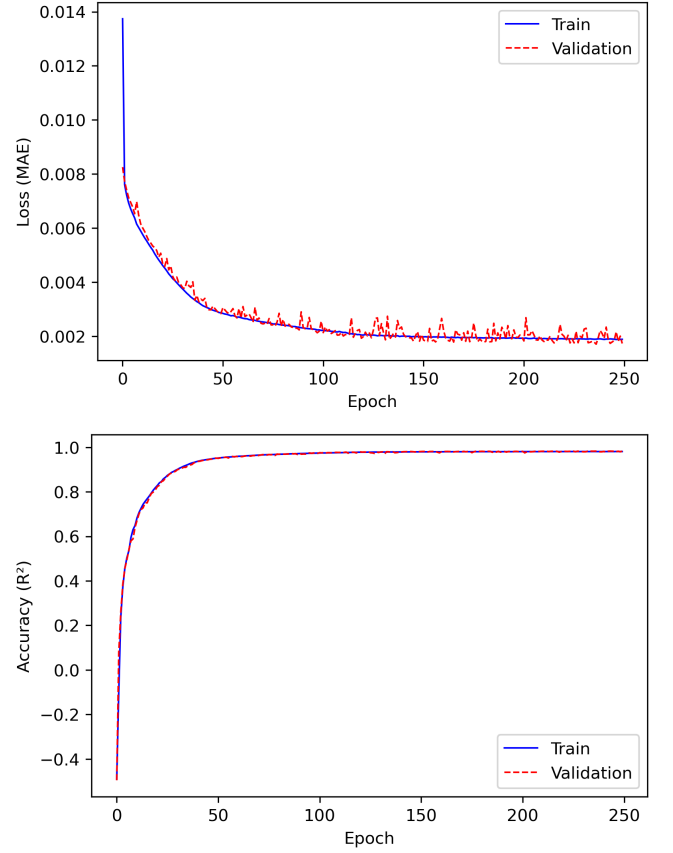

FIG. 4. Convergence of the ANN training process evaluated by train and validation loss (top) and accuracy (bottom).

test sets with a ratio of 60%, 20%, and 20%, respectively. The 20% used for testing are the results presented in the manuscript.

The architecture and learning hyperparameters were optimized based on the performance of the training and validation sets by testing a range of hyperparameters, e.g., the number of neurons in the layers, the learning rate, and the batch size. The developed network includes three hidden layers, each with 50 neurons, as shown in Figure 3.

The network was trained for a total of 250 epochs using the stochastic gradient decent optimizer with an initial learning rate of 0.001, which was reduced by 10% after 10 and 150 epochs. Also, the optimum batch size was found to be 8 geometric states during each training iteration. Initial weights of the network were also optimized by selecting the best weights from 50 training trials. Training and validation performance was assessed based on a regression loss calculated as the mean absolute error (MAE), and an accuracy calculated as the coefficient of determination ( $R^2$ ), given by Equations 15 and 16, respectively. The results are shown in Fig. 4.

$$MAE(t, p) = \frac{1}{n} \sum_{i=1}^n |t_i - p_i| \quad (15)$$

$$R^2(t, p) = 1 - \frac{\sum_{i=1}^n (t_i - \hat{p}_i)^2}{\sum_{i=1}^n (t_i - \bar{t})^2} \quad (16)$$

where  $t$  and  $p$  are the ground-truth and predicted vectors, respectively, with  $n$  examples, and  $\bar{t}$  is the average value of  $t$ .

The ANN was relatively small requiring minimal computational power. Using a CPU (3.20 GHz Intel Core i7-8700), The training process was completed in 5 minutes, and prediction using the trained model was achieved in less than a second for the entire test set.

As discussed in the main paper, the time-dependent aspects of the phenomena cannot be captured with geometrical measures only. Such aspects correspond to the geometrical state data at higher  $Ca$  flows, as presented in Figure 2. Units of time are commonly introduced by the the surface tension and viscosity of the flowing fluids. Since  $Ca$  includes these effects it is the natural parameter to use to supplement the geometric state variables with another measure that can capture time dependent aspects. Therefore, we re-trained a network with all 25,906 geometric states using the 4 Minkowski functionals and  $Ca$  as input. The results are provided in Figure 5. The additional time parameter did not improve the results. Large absolute error remained for the high  $Ca$  flows suggesting that a single time scale parameter cannot capture the time dependent phenomena. Such results are supported by red noise observed during multiphase flow experiments [14].

- 
- [1] F. Blake, The resistance of packing to fluid flow, Transactions of the American Institute of Chemical Engineers **14**, 3 (1922).
  - [2] J. Kozeny, Über kapillare leitung der wasser in boden, Royal Academy of Science, Vienna, Proc. Class I **136**, 271 (1927).
  - [3] J. Bear, *Dynamics of fluids in porous media* (Courier Corporation, 1988).
  - [4] R. Bird, W. Stewart, and E. Lightfoot, *Transport Phenomena* (J. Wiley, 2002).
  - [5] A. Sheppard, S. Latham, J. Middleton, A. Kingston, G. Myers, T. Varslot, A. Fogden, T. Sawkins, R. Cruikshank, M. Saadatfar, *et al.*, Techniques in helical scanning, dynamic imaging and image segmentation for improved quantitative analysis with x-ray micro-ct, Nuclear Instruments and Methods in Physics Research Section B: Beam Interactions with Materials and Atoms **324**, 49 (2014).
  - [6] A. P. Sheppard, R. M. Sok, and H. Averdunk, Techniques for image enhancement and segmentation of tomographic images of porous materials, Physica A: Statistical mechanics and its applications **339**, 145 (2004).
  - [7] D. Pirrie, A. R. Butcher, M. R. Power, P. Gottlieb, and G. L. Miller, Rapid quantitative mineral and phase analysis using automated scanning electron microscopy (qemscan); potential applications in forensic geoscience, Geological Society, London, Special Publications **232**, 123 (2004).
  - [8] M. Shabaninejad, R. Marathe, J. Middleton, and A. Fogden, Micro-ct pore-scale analysis of low salinity recovery from reservoir sandstones, in *77th EAGE Conference and Exhibition 2015* (2015).
  - [9] M. Shabaninejad, J. Middleton, S. Latham, and A. Fogden, Pore-scale analysis of residual oil in a reservoir sand-

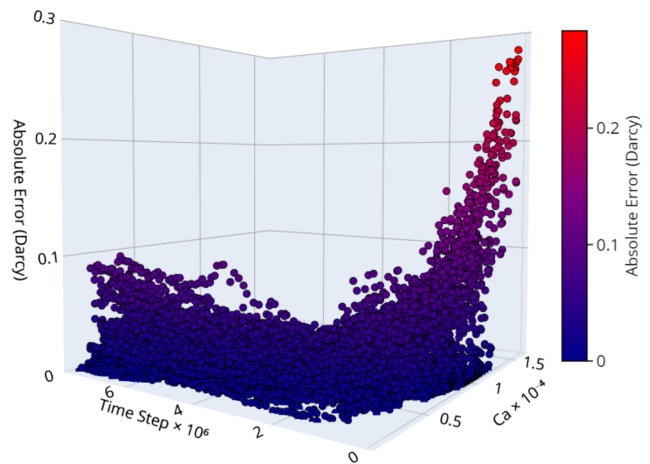

FIG. 5. Absolute error for all 25,906 geometrical states with ANN input as the 4 Minkowski functionals and Capillary number.

- stone and its dependence on water flood salinity, oil composition, and local mineralogy, Energy & Fuels **31**, 13221 (2017).
- [10] S. Latham, T. Varslot, A. Sheppard, *et al.*, Image registration: enhancing and calibrating x-ray micro-ct imaging, Proc. of the Soc. Core Analysts, Abu Dhabi, UAE, 1 (2008).
- [11] K. Askvik, S. Høiland, P. Fotland, T. Barth, T. Grønn, and F. Fadnes, Calculation of wetting angles in crude oil/water/quartz systems, Journal of colloid and interface

- science **287**, 657 (2005).
- [12] B. Jańczuk, E. Chibowski, and T. Białopiotrowicz, Interpretation of the contact angle in quartz/organic liquid film-water system, *Journal of colloid and interface science* **102**, 533 (1984).
  - [13] S. Iglauer, C. Pentland, and A. Busch, Co<sub>2</sub> wettability of seal and reservoir rocks and the implications for carbon geo-sequestration, *Water Resources Research* **51**, 729 (2015).
  - [14] C. Spurin, M. Rücker, M. Moura, T. Bultreys, G. Garfi, S. Berg, M. J. Blunt, and S. Krevor, Red noise in steady-state multiphase flow in porous media, *Water Resources Research* **58**, e2022WR031947 (2022).
